# Supplementary material for: Bigger is Faster in the Adaptive Immune Response
Source: arXiv:2510.09678 ancillary file (2025-10-08)
Supplement: Supplementary file 1 [file Bigger_is_Faster_in_the_Scalable_Adaptive_Immune_Response_2024_supplement.pdf]

# Bigger is Faster in the Adaptive Immune Response

Jannatul Ferdous,<sup>1\*</sup> G. Matthew Fricke,<sup>1,2</sup> Judy L. Cannon,<sup>3</sup> Melanie E. Moses,<sup>1,4,5</sup>

<sup>1</sup>Department of Computer Science, The University of New Mexico, Albuquerque, USA

<sup>2</sup>Center for Advanced Research Computing, Albuquerque, USA

<sup>3</sup>Molecular Genetics and Microbiology, The University of New Mexico, Albuquerque, USA

<sup>4</sup>Department of Biology, The University of New Mexico, Albuquerque, USA

<sup>5</sup>Santa Fe Institute, Santa Fe, USA

\*To whom correspondence should be addressed; E-mail: jannat@unm.edu.

## S1 Methods

### S1.1 Data Collection and Analysis

Using published data, we create a dataset of lymph node (LN) numbers for 10 species, LN volumes for 16 species, and spleen volumes for 36 species with mass recorded for each species.

The data and references used in our analysis are summarized in Table S1. When published animal **masses** are reported as a range, we use the midpoint in our analysis. We use the median when multiple values are published for LNs of the same species. When animal sex is reported, we use male values, because many studies that specifically report LN sizes for female animals are studying the effects of cancer, which impacts LN volume (5).

We compute the **spleen volume** from the mass using the spleen tissue density (1.1 g/mL (38)).

When published **LN numbers** were given as a range, the upper limit is used in our analysis. We use the median values of the number of LNs reported for multiple strains of mouse. **LN volumes** are approximate estimates for each species, which are obtained using various methodologies in

**Table S1: Published Spleen Volume, Lymph Node Volume and Lymph Node Numbers.**  
Mean values and citations for body mass, spleen volume, lymph node (LN) volume, and LN number used in this paper. The number of lymph nodes (LNs) is the maximum reported value assuming that omissions are more likely than additions.

| Common Name                 | Binomial                          | Animal Mass             | Spleen Vol.                  | LN Vol.                       | #LN (Max) |
|-----------------------------|-----------------------------------|-------------------------|------------------------------|-------------------------------|-----------|
| Lab Mouse                   | <i>Mus musculus</i>               | 24 g (1–3)              | 37 mm <sup>3</sup> (2)       | 2.9 mm <sup>3</sup> (2)       | 32 (4)    |
| Egyptian tomb bat           | <i>Taphozous perforatus</i>       | 27 g (1)                |                              |                               | 24 (5)    |
| Greater Mouse Tailed Bat    | <i>Rhinopoma microphyllum</i>     | 28 g (1)                |                              |                               | 26 (5)    |
| Mongolian Gerbil            | <i>Meriones unguiculatus</i>      | 57 g (1)                |                              |                               | 38 (6)    |
| Hamster                     | <i>Mesocricetus auratus</i>       | 130 g (1)               | 260 mm <sup>3</sup> (7)      |                               | 39 (6)    |
| Egyptian Fruit Bat          | <i>Rousettus aegyptiacus</i>      | 130 g (1)               |                              |                               | 46 (5)    |
| Tree Shrew                  | <i>Tupaia belangeri chinensis</i> | 140 g (8)               |                              | 14 mm <sup>3</sup> (8)        |           |
| Tarsius spectrum            | <i>Tarsius tarsier</i>            | 170 g (1)               | 30 mm <sup>3</sup> (9)       |                               |           |
| Common marmoset             | <i>Callithrix jacchu</i>          | 310 g (9)               | 400 mm <sup>3</sup> (9)      |                               |           |
| Guinea Pig                  | <i>Cavia porcellus</i>            | 380 g (10)              |                              | 4.2 mm <sup>3</sup> (11)      |           |
| Rat                         | <i>Rattus norvegicus</i>          | 320 g (1)               | 720 mm <sup>3</sup> (12)     | 26 mm <sup>3</sup> (13)       | 84 (6)    |
| Central American squirrel   | <i>Saimiri oerstedii</i>          | 610 g (9)               | 860 mm <sup>3</sup> (9)      |                               |           |
| Common squirrel monkey      | <i>Saimiri sciureus</i>           | 660 g (9)               | 900 mm <sup>3</sup> (9)      |                               |           |
| Three-striped night monkey  | <i>Aotus trivirgatus</i>          | 740 g (9)               | 1800 mm <sup>3</sup> (9)     |                               |           |
| Cotton-top tamarin          | <i>Saguinus oedipus</i>           | 790 g (9)               | 1600 mm <sup>3</sup> (9)     |                               |           |
| Northern greater galago     | <i>Galago garnettii</i>           | 800 g (9)               | 2100 mm <sup>3</sup> (9)     |                               |           |
| Grivet                      | <i>Cercopithecus aethiops</i>     | 1.4 kg (9)              | 2900 mm <sup>3</sup> (9)     |                               |           |
| Tufted capuchin             | <i>Cebus apella</i>               | 2.2 kg (9)              | 2300 mm <sup>3</sup> (9)     |                               |           |
| Possum                      | <i>Trichosurus vulpecula</i>      | 2.7 kg (1)              |                              | 200 mm <sup>3</sup> (14)      | 67 (14)   |
| Rabbit                      | <i>Oryctolagus cuniculus</i>      | 3 kg (15)               |                              | 62 mm <sup>3</sup> (15–17)    |           |
| White-faced capuchin        | <i>Cebus capucinus</i>            | 3.1 kg (9)              | 11 000 mm <sup>3</sup> (9)   |                               |           |
| Crab-eating macaque         | <i>Macaca fascicularis</i>        | 3.3 kg (9), 3.4 kg (18) | 6800 mm <sup>3</sup> (9)     | 410 mm <sup>3</sup> (19)      |           |
| Cat                         | <i>Felis catus</i>                | 4.5 kg (20)             |                              | 760 mm <sup>3</sup> (21, 22)  |           |
| Bonnet macaque              | <i>Macaca radiata</i>             | 4.5 kg (9)              | 7300 mm <sup>3</sup> (9)     |                               |           |
| Blue monkey                 | <i>Cercopithecus mitis</i>        | 4.9 kg (9)              | 81 000 mm <sup>3</sup> (9)   |                               |           |
| Black howler                | <i>Alouatta caraya</i>            | 5 kg (9)                | 8800 mm <sup>3</sup> (9)     |                               |           |
| Southern pig-tailed macaque | <i>Macaca nemestrina</i>          | 5.2 kg (9)              | 9600 mm <sup>3</sup> (9)     |                               |           |
| Rhesus macaque              | <i>Macaca mulatta</i>             | 5.2 kg (9)              | 4100 mm <sup>3</sup> (9)     |                               |           |
| Lar gibbon                  | <i>Hylobates lar</i>              | 5.7 kg (9)              | 13 000 mm <sup>3</sup> (9)   |                               |           |
| Japanese macaque            | <i>Macaca fuscata</i>             | 5.8 kg (9)              | 4400 mm <sup>3</sup> (9)     |                               |           |
| Tana River mangabey         | <i>Cercocebus galeritus</i>       | 6 kg (9)                | 5100 mm <sup>3</sup> (9)     |                               |           |
| Collared mangabey           | <i>Cercocebus torquatus</i>       | 5.1 kg (9)              | 8600 mm <sup>3</sup> (9)     |                               |           |
| Mantled howler monkey       | <i>Alouatta palliata</i>          | 6.2 kg (9)              | 44 000 mm <sup>3</sup> (9)   |                               |           |
| Stump-tailed macaque        | <i>Macaca arctoides</i>           | 6.2 kg (9)              | 9300 mm <sup>3</sup> (9)     |                               |           |
| Black-handed spider monkey  | <i>Ateles geoffroyi</i>           | 7.6 kg (9)              | 39 000 mm <sup>3</sup> (9)   |                               |           |
| Koala                       | <i>Phascolarctos cinereus</i>     | 10 kg (23)              |                              | 600 mm <sup>3</sup> (24)      |           |
| Formosan rock macaque       | <i>Macaca cyclopis</i>            | 10 kg (9)               | 7600 mm <sup>3</sup> (9)     |                               |           |
| Olive baboon                | <i>Papio anubis</i>               | 13 kg (9)               | 16 000 mm <sup>3</sup> (9)   |                               |           |
| Yellow baboon               | <i>Papio cynocephalus</i>         | 13 kg (9)               | 17 000 mm <sup>3</sup> (9)   |                               |           |
| Chacma baboon               | <i>Papio ursinus</i>              | 15 kg (9)               | 18 000 mm <sup>3</sup> (9)   |                               |           |
| Dog                         | <i>Canis lupus familiaris</i>     | 22 kg (25)              | 48 000 mm <sup>3</sup> (25)  |                               |           |
| Chimpanzee                  | <i>Pan troglodytes</i>            | 30 kg (9)               | 90 000 mm <sup>3</sup> (9)   |                               |           |
| Sheep                       | <i>Ovis aries</i>                 | 50 kg (25)              | 95 000 mm <sup>3</sup> (25)  |                               |           |
| Dolphin                     | <i>Sotalia fluviatilis</i>        | 60 kg (1)               |                              | 1800 mm <sup>3</sup> (26)     |           |
| Human                       | <i>Homo sapiens</i>               | 62 kg (9, 27)           | 160 000 mm <sup>3</sup> (9)  | 560 mm <sup>3</sup> (28)      | 1200 (29) |
| Gorilla                     | <i>Gorilla gorilla</i>            | 65 kg (9)               | 180 000 mm <sup>3</sup> (9)  |                               |           |
| Goat                        | <i>Capra hircus</i>               | 88 kg (30)              |                              | 210 mm <sup>3</sup> (30)      |           |
| Pig                         | <i>Sus scrofa</i>                 | 120 kg (1)              | 330 000 mm <sup>3</sup> (25) | 2000 mm <sup>3</sup> (31, 32) |           |
| Camel                       | <i>Camelus dromedarius</i>        | 390 kg (33)             |                              | 7700 mm <sup>3</sup> (34)     |           |
| Cattle                      | <i>Bos taurus</i>                 | 540 kg (25)             | 860 000 mm <sup>3</sup> (25) | 4200 mm <sup>3</sup> (35)     |           |
| Horse                       | <i>Equus caballus</i>             | 690 kg (1)              | 950 000 mm <sup>3</sup> (25) |                               | 8000 (36) |
| Elephant                    | <i>Loxodonta africana</i>         | 4500 kg (37)            |                              | 5300 mm <sup>3</sup> (37)     |           |

order to facilitate comparisons, as LNs volumes can vary significantly, even within a single individual, particularly in larger animals. For instance, Qatarnah et al. (29) give ranges from 2 mm to 38 mm for human LN diameter. Sometimes, the total volume of each LN is reported, but often only the width and length, or possibly just length, is reported. To estimate volume, we assume LNs are spherical in the case of a single measurement and ellipsoid in the case of two measurements. This may be a source of error in estimating the LN volume. Publications also vary in the number of samples used. When a publication reports values for multiple LNs or from multiple individuals, we take the median value. Different measurement methods, i.e., imaging vs. physical measurements using calipers, may introduce additional variation in the estimated volumes of LN. Although several sources measure a large subset of LNs in larger animals (Table S1), we are not aware of a complete size estimate for all LNs in any large animal. However, human LN size is particularly well studied, which provides some context to interpret variation in LN size. Typically human LN is estimated to be approximately 1 cm in diameter, and diameters larger than 2 cm are considered abnormal or a sign of a disease (39, 40). We use the mean value of the middle of the range in (41), which is exactly 10.25 mm, and consistent with the 1 cm rule of thumb.

**Validating scaling exponents with data from mice and humans:** The noise and heterogeneity in estimates of LN numbers and volumes contribute to wide confidence intervals in the scaling equations. Since, mice and humans are particularly well studied, we use those species as a check on plausible exponents and on the sensitivity of exponents to noise and bias in data. Humans are 2500 times larger than mice. In Table S1, human spleens are 4300 times larger, LN 190 times larger, and LN number is 37 times larger than those of mice. These increases correspond to the following exponents relating these quantities to mass: spleen volume exponent: 1.05, LN volume exponent: 0.56, LN number exponent: 0.52. The estimated total LN volume in humans compared to mice is 7200 times larger, consistent with a slightly superlinear expo-

41 nent of 1.08. All of these numbers are consistent with the trends we identify using the noisier  
42 data from various less well-studied animals.

### 43 **S1.2 Alternative Hypothesis of the Scaling of Spleen Volume**

44 Although the spleen volume data are consistent with the expectation of linear scaling of spleen  
45 size, we also tested an alternative of nonlinear scaling based on the hypothesis that the total  
46 population of T cells and B cells should be proportional to mass  $M$ , multiplied by a logarithmic  
47 term ( $\ln(cM)$ ,  $c$  = arbitrary constant,  $M$  = animal body mass) (42). This assumes that the  
48 number of T cells in each clonal line (that recognize a specific antigen) is proportional to  $M$ ,  
49 and the diversity of T cell clones increases logarithmically with  $M$  based on the diversity of  
50 receptors expected by shape-space theory (43, 44). This prediction is consistent with humans’  
51 slightly larger T cell repertoire compared to mice (45–48).

52 Including a logarithmic term in the regression results in a best-fit exponent of  $\hat{\mu} = 0.99$ . The  
53 Akaike’s Information Criterion (AIC) (49) values for the models with and without logarithmic  
54 terms are 23 and 21, respectively. The lower AIC value slightly favors the model without loga-  
55 rithmic terms, but with such close AIC values, the theorized logarithmic term to accommodate  
56 greater lymphocyte diversity in larger animals also is plausible.

### 57 **S1.3 Statistical Analysis**

58 We estimated the parameters(e.g., exponent) through nonlinear least squares regression in Python  
59 using `scipy.optimize.curve_fit`. We assessed the goodness of fit for our models  
60 through  $R^2$  using `sklearn.metrics.r2_score`. AIC values were computed directly from  
61 the residual sum of squares (RSS) as

$$AIC = n \ln\left(\frac{RSS}{n}\right) + 2k$$

Here  $n$  is the number of observations and  $k$  is the number of fitted parameters. We computed  $p$ -values using a two-tailed t-test, with standard errors estimated from the covariance matrix returned by nonlinear least-squares fitting.

#### S1.4 Derivation of Initial and Mean First Contact Times

Table S2: **Notation** Variables used in this work.

|                      |                                                                                     |
|----------------------|-------------------------------------------------------------------------------------|
| $M$                  | Body mass                                                                           |
| $V_{\text{Spleen}}$  | LN volume                                                                           |
| $V_{\text{LN}}$      | LN volume                                                                           |
| $N_{\text{LN}}$      | LN number                                                                           |
| $c$                  | Arbitrary constant                                                                  |
| $N_{\text{DC}}$      | Number of DCs of antigen per type per LN                                            |
| $N_{\text{TC}}$      | Number of T cells of antigen per type per LN                                        |
| $\lambda$            | Mean first-contact time between intra-LN a single cognate DC and a T cell           |
| $t$                  | Time interval for intra-LN cognate DC-T cell random encounter                       |
| $\tau_{\text{init}}$ | Expected value of intra-LN single cognate DC-T cell pair initial first-contact time |
| $\bar{\tau}$         | Mean value of intra-LN cognate DC-T cells first-contact time                        |
| $\mu$                | scaling exponent                                                                    |

We derive mathematical equations to determine the expected first-contact times ( $\tau$ ) between T cells and different numbers of dendritic cells (DCs) carrying antigen within LNs. We follow the assumptions and approach in Perelson and Wiegel (42) and the Brownian motion model of contact time detailed in Celli et al. (50).

**Assumption 1.** *We assume encounter times are memoryless, and therefore, exponentially distributed. Specifically, if the number of T cells that recognize a given antigen in a LN is  $N_{\text{TC}}$ , then the probability that one DC chosen at random encounters any of the cognate T cells in time  $t$ ,  $P(T_t)$ , can be modeled with an exponential distribution (50),*

$$P(T_t) = \frac{N_{\text{TC}}}{\lambda} e^{-\frac{t N_{\text{TC}}}{\lambda}}$$

Note that we experimentally validated that the assumption that contact times are exponentially distributed is reasonable. We found that in all simulations, the exponential fit was better than a normal distribution fit according to the sum square error (SSE) and AIC (see Figure 3 and Table 2 in (51))

**Definition 1.**  $\lambda$  is the mean contact time between a single searcher and a single target within a volume  $V$ . Celli et al. (50) showed that  $\lambda \propto V$ .

**Derivation 1** (General Scaling Formula for Expected Initial First Contact Time). *The expected initial first contact time is equal to the mean first contact time between a single searcher and a single target in a volume divided by the product of the number of searchers and the number of targets present in the volume.*

Given there are  $N_{DC}$  targets and  $N_{TC}$  searchers, then from Assumption 1, the probability that at least one searcher encounters a target between time 0 and time  $t$  is,

$$P(T < t) = \frac{N_{DC}N_{TC}}{\lambda} e^{-\frac{tN_{DC}N_{TC}}{\lambda}}$$

To obtain the expected encounter time, we integrate over all time,

$$\tau_{init} = \int_0^{\infty} \frac{tN_{DC}N_{TC}}{\lambda} e^{-\frac{tN_{DC}N_{TC}}{\lambda}} dt$$

$$\tau_{init} = \frac{\lambda}{N_{DC}N_{TC}}$$

Derivation 1 states that the expected first contact time is inversely proportional to the product of the number of T cells and DCs. In other words, as the product of these two quantities increases, the expected first contact time decreases.

**Assumption 2.** *To model the initial and mean first contact time, we make the parsimonious assumption that T cells and DCs are initially uniformly distributed within the T cell zone of the LN.*

**Derivation 2** (General Scaling Formula for the Mean First Contact Time). *The mean time a searcher takes to make first contact with a target scales as volume divided by the number of targets.*

From Definition 1  $\lambda$  scales with volume  $V$ . From Assumption 2 the cells are uniformly distributed. Following Perelson and Weigel (42), the time to find a target is inversely proportional to the number of targets ( $N_{DC}$ ), yielding:

$$\bar{\tau} \propto \frac{V}{N_{DC}}$$

**Assumption 3.** *In our analytic model,  $N_{TC}$  refers to the number of naive T cells of a particular specificity within a single lymph node. Although naive T cells are found throughout the body, lymph nodes are the primary sites of antigen presentation and activation. We therefore assume a roughly constant T-cell density across nodes whose number scales as  $M^{1/2}$ , yielding  $N_{TC} \propto M^{1/2}$ . In order to model search times within a LN, we assume that the number of T cells of each clonal line in an animal is proportional to  $M$ , and therefore  $N_{TC}$  is proportional to  $M^{\frac{1}{2}}$  in each of its  $M^{\frac{1}{2}}$  LNs.*

**Assumption 4.** *Perelson and Wiegel (42) predict that the volume of a LN ( $V_{LN}$ ) scales as  $M^{\frac{1}{2}} \ln(cM)$  this is to accommodate the greater clonal diversity of larger mammals.*

**Derivation 3** (Initial First Contact Time Between Cognate T Cell and DC Within the LN). *the expected initial first contact time between cognate populations of DCs and T cells scales logarithmically with mass divided by the number of DCs, i.e.,*

From Definition 1 we have  $\lambda \propto V_{LN}$  and from Assumption 4 we have  $V_{LN} \propto M^{\frac{1}{2}} \ln(cM)$ , therefore

$$\lambda \propto M^{\frac{1}{2}} \ln(cM)$$

Substituting  $\lambda$  into Derivation 1 and  $M^{\frac{1}{2}}$  for  $N_{TC}$  from Assumption 3, yields the expected initial

117 first contact time in a LN:

$$\begin{aligned}\tau_{\text{init}} &= \frac{\lambda}{N_{\text{DC}} N_{\text{TC}}} \\ &\propto \frac{M^{\frac{1}{2}} \ln(cM)}{N_{\text{DC}} M^{\frac{1}{2}}} \\ \tau_{\text{init}} &\propto \frac{\ln(cM)}{N_{\text{DC}}}\end{aligned}$$

118 We derive  $\tau_{\text{init}}$  for two relevant bounding cases: 1) the number of DCs responding to in-  
 119 fection is proportional to  $M$  (i.e., a constant density of DCs respond to a systemic infection).  
 120 Therefore, the number in a single LN is assumed proportional to  $M^{\frac{1}{2}}$  in each of the  $M^{\frac{1}{2}}$  LN. 2)  
 121 when the number of DCs responding to an infection is constant, reflecting a localized infection.  
 122 For each of these boundary cases, we derive the expected initial first contact time and the mean  
 123 first contact time.

124 **Prediction 3.1** (Initial First Contact with Constant Density of DCs). *The density of cognate DC*  
 125 *is constant with respect to  $M$ , and the number of LNs scales with  $M^{\frac{1}{2}}$ . Hence the number of*  
 126 *DCs ( $N_{\text{DC}}$ ) per LN scales with  $M^{\frac{1}{2}}$ . Substituting the scaling of DCs in Derivation 3, we have*  
 127  $N_{\text{DC}} \propto M^{\frac{1}{2}} \Rightarrow \tau_{\text{init}} \propto M^{-\frac{1}{2}} \ln(cM).$

128 **Prediction 3.2** (Initial First Contact with Constant Number of DCs). *Similarly, if the number of*  
 129 *DCs presenting cognate antigen in LNs is constant as  $M$  increases then we substitute a constant*  
 130 *for  $N_{\text{DC}}$  in Derivation 3. Then the expected initial first-contact time scales logarithmically with*  
 131 *mass, i.e.,  $N_{\text{DC}} = C \Rightarrow \tau_{\text{init}} \propto \ln(cM).$*

132 In addition to modeling the initial first time for a T cell to contact its cognate DC, we  
 133 also consider the mean first-contact times ( $\bar{\tau}$ ) for a typical T cell to contact its cognate antigen-  
 134 bearing using a constant density of T cells and DCs, following the approach outlined by Perelson  
 135 and Wiegel (42). Consistent with their predictions, we find a logarithmic increase in  $\bar{\tau}$  (Figure 3,



panel A, top blue line). Considering the other extreme case of a constant number of DCs carrying the relevant antigen, we predict mean contact times to increase with  $M^{\frac{1}{2}} \ln(cM)$ .

**Derivation 4** (Mean First Contact Time Between Cognate T Cell and DC Within the LN). *The mean time a T cell takes to make first contact with a particular DC displaying cognate antigen when the LN volume scales with mass, scales as  $M^{\frac{1}{2}} \ln(cM)$  divided by the number of DCs, i.e.,*

$$\bar{\tau} \propto \frac{M^{\frac{1}{2}} \ln(cM)}{N_{DC}}$$

The result follows immediately from substituting the value of  $V_{LN}$  from Assumption 4 into Derivation 2.

**Prediction 4.1** (Mean First Contact with Constant Density Scaling). *The density of cognate DCs is constant with respect to  $M$ , and the number of LNs scales with  $M^{\frac{1}{2}}$ . Therefore,  $N_{DC}$  per LN scales with  $M^{\frac{1}{2}}$ . Substituting the scaling of DCs in Derivation 4, the expected mean first-contact time scales logarithmically with mass, i.e.,  $N_{DC} \propto M^{\frac{1}{2}} \Rightarrow \bar{\tau} \propto \ln(cM)$ .*

**Prediction 4.2** (Mean First Contact with Constant Number Scaling). *Similarly, if the number of DCs presenting cognate antigen in LNs is constant as  $M$  increases, then we substitute a constant for  $N_{DC}$  in Derivation 4. Then the expected mean first-contact time scales as mass to the one-half power, i.e.,  $N_{DC} = C \Rightarrow \bar{\tau} \propto M^{\frac{1}{2}} \ln(cM)$ .*

Table S3 shows the predicted values of mean first contact times  $\bar{\tau}$  for both systemic and localized infections. For larger mammals,  $\bar{\tau}$  is predicted to range from several days to weeks, which is far longer than the observed times for T cells to find their DC targets in the LN and replicate to detectable numbers. Thus, we suggest that the mean first contact time is not relevant for initiating the adaptive immune response, although it may be an important factor in determining the magnitude or timing of the peak T cell response.

Table S3: **DC-T Cell Mean First Contact Times** considering 2 cases: i) assuming the number of DC in LN scales with  $M^{0.5}$  (constant density of antigen-bearing DC from a systemic infection) and ii) a constant number of DC in LN ( $N_{DC} = \text{Constant}$ ). We estimate times for each case, considering that T cells move in using either *Brownian motion* or a *persistent random walk*.

| Mass          | $N_{DC} \propto M^{\frac{1}{2}}$ |                        | $N_{DC} = \text{Constant}$ |                        |
|---------------|----------------------------------|------------------------|----------------------------|------------------------|
|               | Brownian Motion                  | Persistent Random Walk | Brownian Motion            | Persistent Random Walk |
| 24 g (Mouse)  | 1 d                              | 0.80 d                 | 0.65 d                     | 0.49 d                 |
| 1 kg          | 2.3 d                            | 1.7 d                  | 9.1 d                      | 7 d                    |
| 62 kg (Human) | 3.6 d                            | 2.9 d                  | 120 d                      | 89 d                   |

Figure S1 shows that how both predicted and simulated  $\bar{\tau}$  scale for systemic and localized infections. For systemic infection where  $N_{DC}$  scale as  $M^{\frac{1}{2}}$ , the prediction is  $\bar{\tau} \propto M^0 \ln(cM)$  and the fit from the simulation gives  $\bar{\tau} \propto M^{0.01} \ln(cM)$ . The slight increase in  $\bar{\tau}$  for systemic infection in Figure S1 indicates that  $\bar{\tau}$  increases logarithmically with mass, despite the near-zero exponent of M.

For a localized infection ( $N_{DC} = \text{Constant}$ ),  $\bar{\tau}$  scales as  $M^{\frac{1}{2}}$ . This intuitive outcome arises because the time for the rare fortunate *first* contact is expedited when more T cells are present. However, the advantage of a large population doesn't benefit the *typical* T cell, as they don't experience a faster encounter.

### S1.5 Mean First Contact Times Within an Abstract Volume

If the density of T cells and DCs are kept constant,  $N_{TC} \propto N_{DC} \propto V$ , then from Derivation 1,

$$\tau_{\text{init}} \propto V^{-1} \quad (\text{S1})$$

That is, given a constant density of T cells and DCs, the time for the initial first contact between a T cell and a DC is inversely proportional to the LN volume. When the density of the targets is constant,  $N_{DC} \propto V$ , then from Derivation 2, the mean first contact time is constant with respect

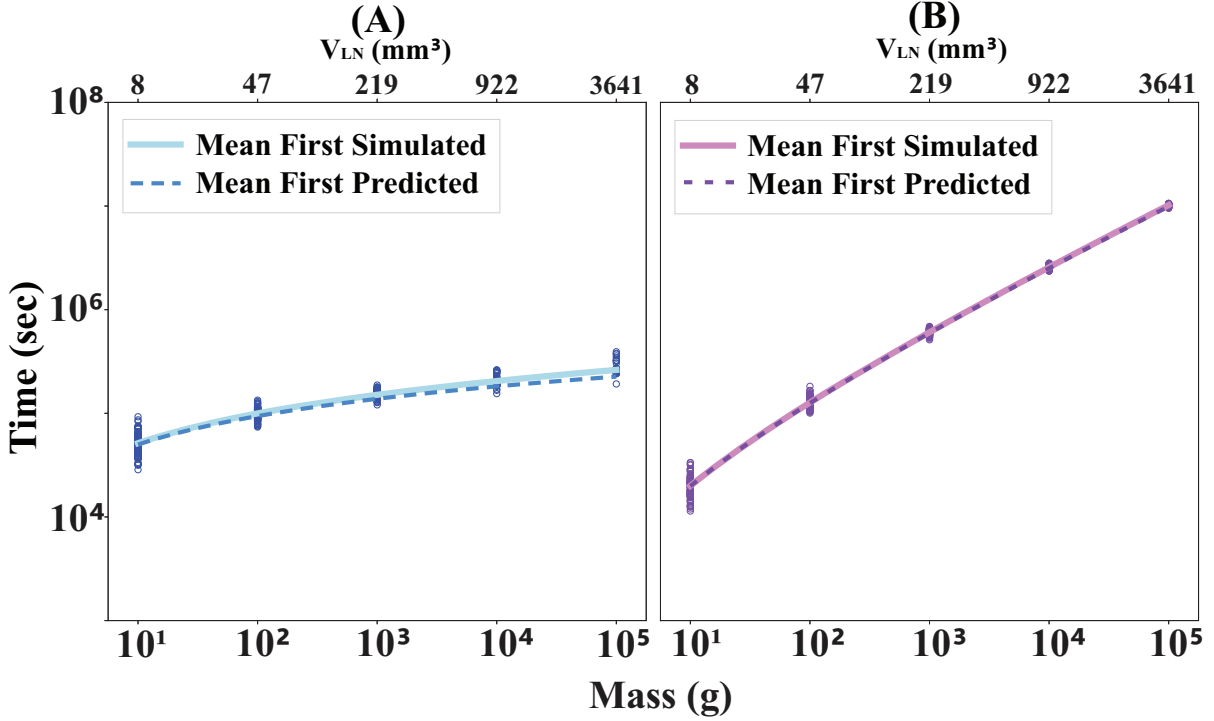

Figure S1: **Theoretical Predictions for Mean Search Time vs Animal Mass are Consistent with Simulations of T Cell Contact Times in Lymph Nodes.** **Panel A:** For systemic infection ( $N_{DC} \propto M^{\frac{1}{2}}$ ), the predicted mean first-contact time is  $\bar{\tau} \propto M^\mu \ln(cM)$  with,  $\mu = 0$  (dashed blue line). The best fit (solid blue line) for the corresponding simulated data (blue points) gives the exponent  $\hat{\mu} = 0$  (95% CI [-0.01, 0.01]). **Panel B.** For small localized infections ( $N_{DC} \propto M^0$ ), the predicted mean first-contact time, is  $\bar{\tau} \propto M^\mu \ln(cM)$  with  $\mu = 0.5$  (dashed purple line). The best fit (solid purple line) to the simulated data (purple points) gives the value for the exponent,  $\hat{\mu} = 0.50$  (95% CI [0.49, 0.51]). The simulations for all these two cases are consistent with theoretical predictions.

172 to volume, in sharp contrast to  $t_{init}$ :

$$\bar{\tau} \propto V^0 \quad (\text{S2})$$

173 These simple equations predict that if a constant density of searchers looks for a constant density  
 174 of targets in a larger three-dimensional space, the first contact will happen faster, the speedup  
 175 will be proportional to the volume in which the search takes place, and the mean first contact  
 176 will be constant across all LN volumes. We simulate a uniform random distribution of searchers  
 177 and targets in Figure 4 from (51) which shows that initial first contact times scale inversely

proportional to volume. Figure S1 shows that for uniform random distribution of searchers and targets, the mean first contact is constant across volume as predicted by Equation (S1) and Equation (S2). The inverse linear dependence of  $\tau_{init}$  on both  $N_{DC}$  and  $N_{TC}$  occurs because each searcher is assumed to search for each target independently. This assumption holds for searchers moving with a random walk in a three-dimensional space, leading to an exponential distribution of search times (see Figure 3 and Table 2 in (51))

## S1.6 Agent Based Model

To validate our mathematical model, we implement an agent based model, termed Initial first contact time (IFCT) using the MASON libraries (52) in Java. The model simulates two types of agents - T cell (searchers) and DC (targets). Both are uniformly distributed within a cubic representation of a LN. LN space is modeled as a continuous Cartesian grid in three dimensions with fixed reflective boundaries.

IFCT model is run as a discrete-time simulation, with each time step representing one second. At the beginning of each simulation run, a predefined number of T cells and DCs are initialized (see Section S1.7). The positions of DCs are static throughout the simulation. T cells, on the other hand, move in each time step with either Brownian motion or a persistent random walk, which was modeled from empirical data in Fricke et al. (53) (Note that previous analysis (42, 50), assumed Brownian motion). Table S3 contains the results from both types of walks, demonstrating their similarity. Figure 3 and Figure S1 shows the result of Brownian motion. Following the hypothesis given in (42), we assume T cells scale  $\propto M^{\frac{1}{2}}$ . We model T cell motion without considering collisions so that T cells pass through each other.

We run the IFCT model for the two bounding cases, one in which  $N_{DC} \propto M^0$ , i.e. a constant, and another where  $N_{DC} \propto M^{\frac{1}{2}}$ . Each case is simulated for five different animal mass ( $M$ ) values. For each  $M$ , we run 100 experimental replicas for each combination of factors

Table S4: Experimental factor levels used in the ABM experiments.

| Mass (M) |                                   | 10 g                | $1 \times 10^2$ g  | $1 \times 10^3$ g   | $1 \times 10^4$ g   | $1 \times 10^5$ g    |
|----------|-----------------------------------|---------------------|--------------------|---------------------|---------------------|----------------------|
| $V_{LN}$ | $\propto M^{\frac{1}{2} \ln(cM)}$ | 7.3 mm <sup>3</sup> | 46 mm <sup>3</sup> | 220 mm <sup>3</sup> | 920 mm <sup>3</sup> | 3600 mm <sup>3</sup> |
| $N_{TC}$ | $\propto M^{\frac{1}{2}}$         | 20                  | 63                 | 200                 | 630                 | 2000                 |
| $N_{DC}$ | $\propto M^{\frac{1}{2}}$         | 80                  | 250                | 800                 | 2500                | 8000                 |
| $N_{DC}$ | = constant                        | 200                 | 200                | 200                 | 200                 | 200                  |

where the initial distribution of the T cells and DCs are stochastic. We assume that there is a contact between a T cell and DC when their centers are within 10 microns. The simulation result from IFCT model confirms that the distribution of contact times is exponential, an assumption that underpins the theoretical derivation.

### S1.7 Fitting Exponents to data generated by the ABM

The first contact time between any cognate DC and T cell initiates the adaptive immune response. To compute exponent  $\mu$  over M in the initial first-contact time formulas from the experimental data Predictions 3.1 and 3.2, we first generate a generic formula by combining Prediction 3.1 and Prediction 3.2 as follows,

$$\tau \propto M^\mu \ln(cM)$$

For ease of presentation, we convert the generic formula to base 10 as follows,

$$\begin{aligned} \log_{10}(\tau) &= \log_{10}(aM^\mu \ln(cM)) \\ &= \log_{10}(a) + \mu \log_{10}(M) + \log_{10}(\ln(c) + \log_{10}(M) \ln(10)) \end{aligned}$$

If we set,  $C_1 = \log_{10} a$  and  $C_2 = \ln(c)$  then,

$$\log_{10}(\tau) = C_1 + \mu \log_{10}(M) + \log_{10}(C_2 + \log_{10}(M) \ln(10))$$

and exponentiating,

$$\tau = 10^{C_1 + \mu \log_{10}(M) + \log_{10}(C_2 + \log_{10}(M) \ln(10))}$$

Table S5: **DC-T Cell *Initial First Contact Times*** Following Perelson model considering 2 cases: i) constant density of antigen-bearing DC from a systemic infection and ii) a constant number of DC in LN ( $N_{DC} = M^0$ ). We estimate times for each case, considering that T cells move using a *persistent random walk*.

| Mass          | $N_{DC} \propto M^{\frac{1}{2}}$ | $N_{DC} = M^0$ |
|---------------|----------------------------------|----------------|
| 24 g (Mouse)  | 28 min                           | 14 min         |
| 1 kg          | 9.1 min                          | 28 min         |
| 62 kg (Human) | 1.6 min                          | 60 min         |

Perelson and Wiegel in (42) ask how long it takes for a single B cell to encounter a T cell given assumptions Equations (1) and (2). [FIXME] This approach considers the mean time it takes any particular B cell to encounter a T cell. They proposed a formula for the mean first contact time,  $\bar{\tau}$ , which a B cell needs to make first contact with some T cell of the complementary clone should scale like,

$$\bar{\tau} \propto \frac{V_{LN}}{N_{TC}} \quad (S3)$$

We used the same method to compute the fitted exponent value for the mean first contact time in our code, as described above for the initial first contact time.

## S2 IFCT Model Validation

We used experimental data from De Boer et. al. (54) to validate that our IFCT simulations provide biologically realistic estimates of the times for T cells to first contact their cognate DC. We compared contact times and resulting peak T cell populations from two models. We compare our IFCT model that explicitly represents the time that each T cell takes to contact its cognate DC to a Median model that uses the median first contact time as the estimated contact time for all T cells to contact their cognate DC. We show that the median contact time that we estimate from our IFCT model is consistent with data and assumptions in (54). We also show that explicitly considering the variation in contact times leads to larger estimated peak T cell populations.

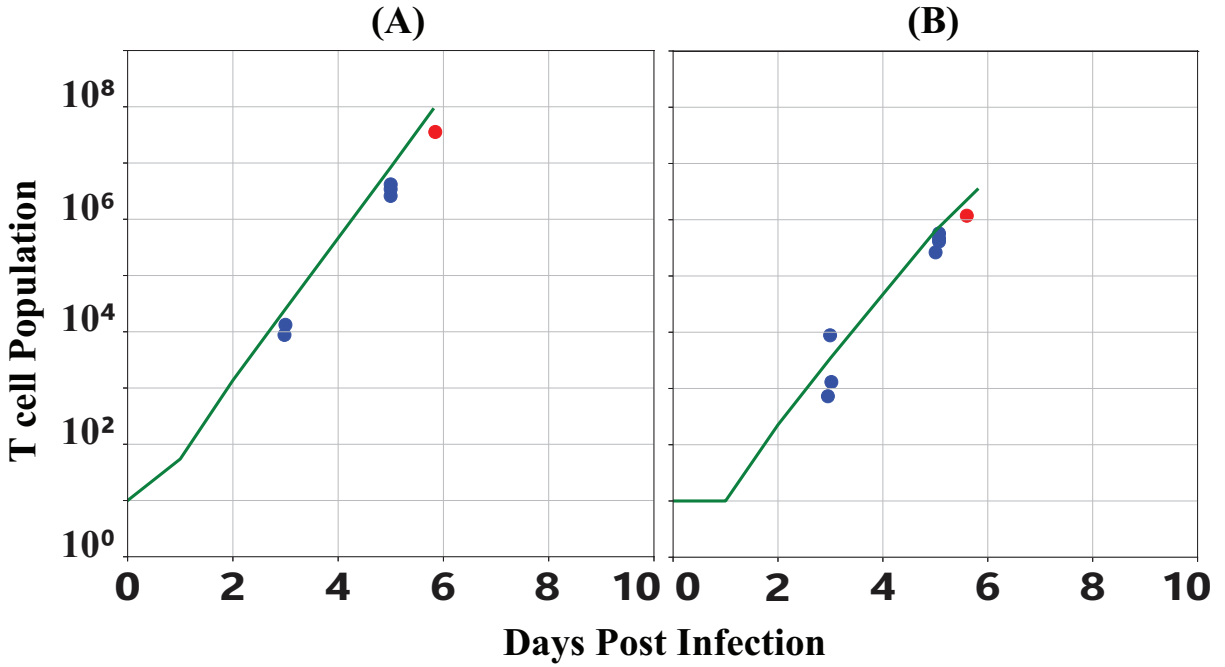

Figure S2: **T Cell Population Growth From the IFCT Model Compared to Empirical Data and Median Model.** Panel A depicts the T cell population over time in response to epitope NP118 for 5.8 days post-infection and Panel B depicts the same for epitope GP283 for 5.6 days post-infection. Blue data points are empirical data from (54) representing T cell populations at specified time points post-infection. The red data point is the Median model prediction of the peak T cell population. The green line shows the estimates from the IFCT model parameterized by data in (54).

We set the parameters of our IFCT simulation to correspond to the empirical system modeled in (54): 60 precursor T cells searching for DCs in a spleen of volume  $46 \text{ mm}^3$  for two different epitopes (NP118 and GP283). We note that these empirical findings are close to our scaling estimate that a 37 mm LN should contain 63 T cells (Table S1).

Following (54), we consider four post-infection phases from the initial infection until the T cells reach their peak population:

1. travel time for a T cell and antigen carrying cognate DCs to travel to the spleen ( $t_{travel}$ )
2. initial contact time between the T cells and their cognate antigen-bearing DC ( $\tau_{init}$ )

3. activation time it takes for a T cell to become fully activated upon encountering the cognate DC ( $t_{act}$ )

4. proliferation time it takes for activated T cells to replicate ( $t_{rep}$ ).

We define recruitment time ( $t_{rec}$ ) as

$$t_{rec} = t_{travel} + \tau_{init} + t_{act}$$

The model of the mouse spleen (54), which we call the Median model, uses the same  $t_{rec}$  and the same  $\tau_{init}$  for every T cell. In (54),  $t_{rec}$  was estimated to be 1.2 days for epitope NP118 and 1.7 days for epitope GP283. The model in (54) does not explicitly estimate  $\tau_{init}$ . Here we estimate this time for all T cells as the median of all initial contact times ( $\tau_{init}^{median}$ ) collected from our IFCT model.

In our IFCT simulation, we draw each contact ( $\tau_{init}^i$ ) from our simulation that ranges from 0.47 hrs to 150 hrs (0.019 days to 6.4 days) with a median ( $\tau_{init}^{median}$ ) time of 22 h (0.9 days). The list of first contact times for each simulated T cell is available here: <sup>1</sup>.

To compare the IFCT model to the Median model, we compute the sum of the travel time and activation time ( $t_{travel+act} = t_{travel} + t_{act}$ ) by subtracting the median first contact time  $\tau_{init}^{median}$  from the recruitment time  $t_{rec}$ .

$$t_{travel+act} = t_{travel} + t_{act} = t_{rec} - \tau_{init}^{median}$$

This gives us the summation of travel and activation time to be 6.8 hr and 18.8 hr for NP118 and GP283 epitopes respectively.

We calculate proliferation times ( $t_{rep}$ ) as the inverse of proliferation rates  $r_{rep}$  in (54) given as 2.9 per day for epitope NP118 and 2.6 per day for epitope GP283. Thus  $t_{rep}$  is 0.39 days

---

<sup>1</sup>[https://docs.google.com/spreadsheets/d/1ur3b4BpyfezHVAKFbyul0Y7N\\_X9-QGBA\\_BxZjYZuvsA/edit?usp=sharing](https://docs.google.com/spreadsheets/d/1ur3b4BpyfezHVAKFbyul0Y7N_X9-QGBA_BxZjYZuvsA/edit?usp=sharing)



**Table S6: Parameters and Peak Population estimates from the Median and IFCT models.** The recruitment time and proliferation time are from (54). The travel and activation time ( $t_{travel+act}$ ) represents the corresponding time after subtracting the median first contact time ( $\tau_{init}^{median}$ ) from the recruitment time ( $t_{rec}$ ). Peak T cell populations are after 5.8 days and 5.6 days post-infection for epitope NP118 and GP283 respectively. The median first contact time in the Median model is 22 hr for all T cells and the first contact time is different for every T cell in the IFCT model.

| Parameter                  | Symbol           | Units | NP118 | GP283 |
|----------------------------|------------------|-------|-------|-------|
| Recruitment Time           | $t_{rec}$        | days  | 1.2   | 1.7   |
| Travel and Activation Time | $t_{travel+act}$ | days  | 0.26  | 0.76  |
| Proliferation Time         | $t_{rep}$        | days  | 0.35  | 0.39  |

  

| Peak T cell Population Based on Fits |  |                   |
|--------------------------------------|--|-------------------|
| Median Model Estimation              |  | $3.9 \times 10^7$ |
| IFCT Model Estimation                |  | $9.1 \times 10^7$ |
| Fold increase                        |  | 2.3               |

and 0.35 days for these epitopes. (54) estimated that proliferation stops, reaching the peak population  $t_{peak}$ , at day 5.8 for epitope NP118 and at day 5.6 for epitope GP283. The IFCT model assumes the exponential growth occurs between  $t_{rec}^i$  and  $t_{peak}$ , and we define that remaining time  $t_{rem}^i$  for each T cell  $i$  as follows,

$$t_{rem}^i = t_{peak} - t_{travel+act} - \tau_{init}^i$$

We continue this until  $t_{rem}^i \geq t_{rep}$  so that we only count the T cells that complete proliferation before the  $t_{peak}$ . The total number of T cells ( $N_{peak}$ ) at  $t_{peak}$  was calculated in the IFCT model as

$$N_{peak} = \sum_{i=1}^n e^{t_{rem}^i * r_{rep}}$$

In Figure S2, we show the correspondence of the mean T cell population dynamics of 10 simulations from the IFCT model with data from (54) over time and with data from Median Model at  $t_{peak}$ . Table S6 shows that the IFCT estimated peak T cell populations at  $t_{peak}$  are twice as high as the Median model.

This analysis shows two things. First, the median first contact time  $\tau_{init}^{median}$  calculated from our IFCT simulations is consistent with times in (54) when the recruitment time  $t_{rec}$  is broken down into travel, first contact, and activation phases. Second, when we model the process in which each T cell finds its cognate antigen and then proliferates exponentially, the population of T cells begins growing earlier and reaches a higher peak compared to the modeling of the average T cell in prior work.

## **S2.1 Analysis of IFCT model effect on peak T cell population across different lymph node sizes**

We further analyze T cell population growth for systemic infection which assumes a constant density of DC. For simplicity, we don't consider the travel time and activation time; we model the proliferation that begins after the first contact time  $\tau_{init}$  between T cell and DC and ends when the T cell population reaches its peak at  $t_{peak}$ , giving us  $t_{rem}$  as

$$t_{rem} = t_{peak} - t_{init}$$

We compare the population in the Median and IFCT models for two cases: a smaller LN of 46 mm<sup>3</sup> with 60 T cells and a larger LN of 3600 mm<sup>3</sup> with 1733 T cells. The LN size ( $V_{LN}$ ) and its corresponding T cell numbers ( $N_{TC}$ ) are determined based on Assumption 4 ( $V_{LN} \propto M^{0.5} \ln(cM)$ ) and Assumption 3 ( $N_{TC} \propto M^{0.5}$ ). We assume the population reaches its peak at  $t_{peak} = 8$ th day after the first T cell contacts its cognate DC.

Figure S3 illustrates that the IFCT model begins replication immediately after the initial T cell contact (0.02 days for the smaller LN and 0.0015 days for the larger LN) which captures the critical early interactions between T cells and DC. In contrast, in the Median model, the initiation of the T cell replication is delayed until the median contact time (0.9 days for the smaller LN and 2.06 days for the larger LN). Table S7 shows the population at day 4 and day 8 in both models. This early start in the IFCT model is consistent with biological evidence that

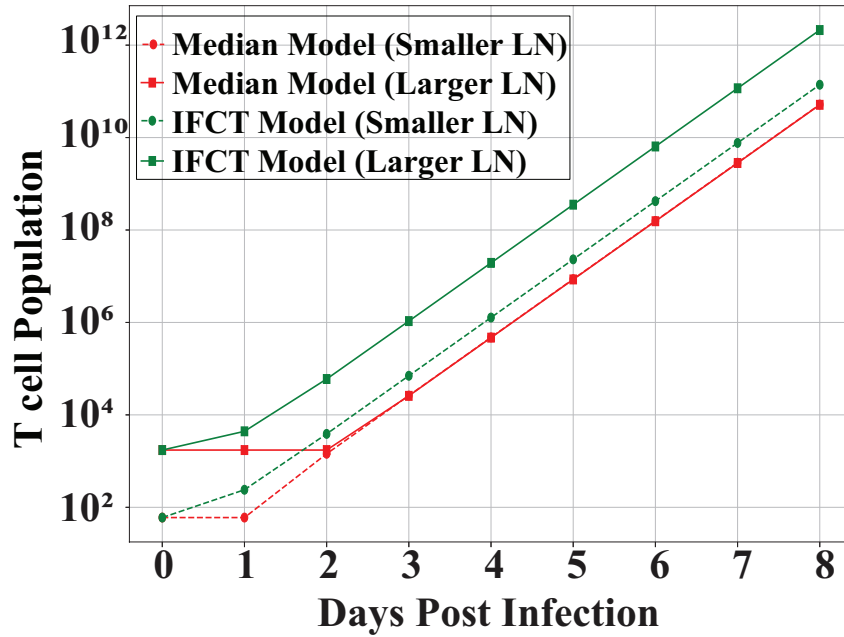

Figure S3: **T Cell Population Comparison Between Simplified Models for Smaller and Larger Lymph Nodes.** The figure compares the log-transformed daywise T cell populations predicted by the Median model and IFCT model upto 8 days of exponential growth. The red dashed line represents the Median prediction for a smaller LN (60 initial T cells), and the red solid line corresponds to the Median prediction for a larger lymph node (1733 initial T cells). The green dashed line represents the IFCT model for a smaller LN (60 initial T cells), and the green solid line corresponds to the IFCT prediction for a larger lymph node (1733 initial T cells).

T cells begin proliferating as soon as they encounter an antigen, a key event in initiating the immune response. As a result, the IFCT model predicts consistently higher T cell populations. By the time the Median model initiates proliferation, the IFCT model predicts 239 T cells in the smaller LN and 59700 T cells in the larger LN, which are 3.98 and 33.67 times higher, respectively, than the Median model's predictions at the median contact times of 0.9 and 2.06 days for smaller and larger LN. This substantial early proliferation in the IFCT model is particularly advantageous in larger LN with more T cells.

The ratio between the IFCT model predictions and the Median model predictions remains approximately proportional over time (2.7-fold higher in smaller LN and 41-fold higher in larger

**Table S7: Comparison of T Cell Population Growth Predictions for Smaller and Larger Lymph Nodes Using Simplified Median and IFCT Models at Day 4 and Day 8.** The table illustrates the median contact time and T cell population estimates after 4 and 8 days for a smaller LN (60 initial T cells) and a larger LN (1733 initial T cells) based on the two models. The Median model assumes simultaneous contact for all T cells, while the IFCT model allows for individual first contact times. X-fold growth represents the ratio between IFCT and Median model predictions for each scenario.

|                            | Smaller LN w/ 60 T cells |                      | Larger LN w/ 1733 T cells |                      |
|----------------------------|--------------------------|----------------------|---------------------------|----------------------|
| Median Contact Time (days) | 0.90                     |                      | 2.1                       |                      |
|                            | After day 4              | After day 8          | After day 4               | After day 8          |
| Median Model Prediction    | $4.8 \times 10^5$        | $5.2 \times 10^{10}$ | $4.7 \times 10^5$         | $5.1 \times 10^{10}$ |
| IFCT Model Prediction      | $1.3 \times 10^6$        | $1.4 \times 10^{11}$ | $1.9 \times 10^7$         | $2.1 \times 10^{12}$ |
| Fold increase              | 2.7                      | 2.7                  | 40                        | 41                   |

LN).

Additionally, Figure S3 shows how incorporating the IFCT predictions for first contact times dramatically increases the predicted peak number of T cells in larger LN. In the traditional Median model, the T cell replication starts earlier in the smaller LN compared to the larger LN because the median first contact time is longer in the larger LN. In contrast, in the IFCT model, the first contact occurs 13.33 times faster in the larger LN (0.0015 days) compared to the smaller LN (0.02 days). Thus, in the IFCT model, the larger LN has more T cells and they begin replicating faster; this early advantage persists, resulting in a 41-fold increase in predicted peak number of T cells in the IFCT model compared to the Median model.

We note that, of course, not every T cell can contact its cognate antigen faster than the median contact time. In fact, the last T cell to contact its cognate DC is slower in the large LN (7.62 vs 3.98 days). However, because of exponential growth, the last contact makes a far smaller contribution to the peak number of T cells. The first T cell has replicated 6 times (generating  $2^6 = 64$  daughter T cells) before the median T cell makes contact, and 20 times (generating  $2^{20} = 1$  million daughter T cells) before the last T cell makes contact. This illustrates why the timing of the first contact is so important - the earliest T cells to contact cognate

DC are by far the most important contributors to the exponentially growing population of T cells.

### **S3 Caveats and Limitations**

There are several caveats to consider in the empirical and modeling work we present here. First, all data we provide are species averages, and many are difficult to estimate from empirical data. Few studies have counted the total number of LN in different species, introducing potential variability. Additionally, estimating LN volumes accurately from one or two length measurements is difficult, particularly in large animals where LN sizes may vary dramatically within individuals. See Section S1 for further details on potential biases from measurements. However, the approximate LN volumes reported in published literature show a clear trend with animal mass, allowing us to understand significant differences in LN size and number. This is validated by comparing data between the best-studied species – humans and mice. The distribution of LN volumes within animals remains a question for future studies.

Our mathematical models and simulations are, of course, simplifications of the complex search processes that occur in LNs. We model the search process as a Brownian random walk in a cube or sphere without considering the crowding or structures that may influence how T cells move in LNs, although we do consider alternate movements that mimic real T cell movement patterns (53) and find that realistic movement decreases search times by only a small percentage (Table 2 in the main file).

The assumption that T cells and DCs are uniformly distributed throughout the T cell zone at any given time is only an approximation. In reality, T cells and DCs enter LNs through lymphatic vessels over time. We simplify the complex dynamics of how T cells bind to different antigens presented by DC by considering only a single clonal line of T cells and a single antigen. It is unclear how many different clonal lines of T cells might match a particular antigen or the

number of antigens DCs present from any given pathogen. There are empirical and theoretical suggestions that the clonal diversity of T cells increases slowly with  $M$ . Figure 2 shows spleen volume, and LN volume scaling could accommodate a linear increase in T cells per clonal line and a logarithmic increase in the number of clonal lines. Still, more data are needed to test this hypothesis.

Because our IFCT model is focused on search times within LN, we do not address other potential causes or consequences of LN size and number. Physiological and anatomical constraints exist on the size, number, and placement of LN. LNs have multiple functions, for example, holding the population of exponentially growing B cells and T cells, which would logically also constrain the minimum size of LN. How these factors influence LN size remains an open question.

Finally, many factors determine the scaling of immune response times that we do not address here. The magnitude and scaling of the times to complete multiple steps in Figure 1 could be affected by the animal's size and metabolism. In particular, the transport of antigen from peripheral tissue to LN by DC would be longer in larger animals if DC speed is constant and LN are lower density and therefore further apart (55). T cells might be expected to replicate more slowly in larger animals, following the typical quarter-power slowdown with body mass. This would mean it would take 7 times longer for T cells to replicate in humans vs. mice, but we are aware of no evidence of such systematic differences.

Perelson has hypothesized that LN might be metabolically privileged locations with sufficient metabolic resources for T cells to replicate as fast in humans as mice (42). Finally, the timing of adaptive immune responses is intricately connected to innate immune responses, which have their own scaling properties, e.g., those investigated in (56). Others have identified differences in components of immune response across species (57, 58), suggesting a complex relationship between animal size and immune response that is important for translating obser-

366 vations between laboratory animals, animal sources of zoonotic disease and humans. While we  
367 leave a full accounting of factors that contribute to the scaling of adaptive immune response  
368 times to future work, the analysis we present here points to the decentralized architecture of the  
369 lymphatic network with sublinear increases in LN size and number with animal size as a key  
370 factor explaining how the adaptive immune response can be nearly as fast in large vs. small  
371 animals.

## 372 References

- 373 1. F. A. Smith, *et al.*, Body mass of Late Quaternary mammals: ecological archives E084-094.  
374 *Ecology* **84** (12), 3403–3403 (2003).
- 375 2. V. Economopoulos, J. C. Noad, S. Krishnamoorthy, B. K. Rutt, P. J. Foster, Comparing the  
376 MRI appearance of the lymph nodes and spleen in wild-type and immuno-deficient mouse  
377 strains. *PLoS One* **6** (11), e27508 (2011).
- 378 3. Body Weight Information for J:NU (007850), [https://www.jax.](https://www.jax.org/jax-mice-and-services/strain-data-sheet-pages/body-weight-chart-007850)  
379 [org/jax-mice-and-services/strain-data-sheet-pages/](https://www.jax.org/jax-mice-and-services/strain-data-sheet-pages/body-weight-chart-007850)  
380 [body-weight-chart-007850](https://www.jax.org/jax-mice-and-services/strain-data-sheet-pages/body-weight-chart-007850).
- 381 4. Y. Kawashima, M. Sugimura, Y.-C. Hwang, N. Kudo, The lymph system in mice. *Japanese*  
382 *Journal of Veterinary Research* **12** (4), 69–78 (1964).
- 383 5. D. Y. Abel-Galil, A.-R. Tawfik, A.-H. Saad, Anatomical and comparative distribution of  
384 lymph nodes in some Egyptian chiroptera. *Scolar. cu. edu. eg* .
- 385 6. Y. Kawashima, The lymph system in rodents. *Japanese Journal of Veterinary Research*  
386 **20** (1-2), 35–36 (1972).

- 387 7. G. H. Friedell, J. D. Sherman, P. G. Rigby, The effect of foreign protein on the blood and  
388 reticuloendothelial system of the hamster. *Blood* **21** (1), 80–88 (1963).
- 389 8. N. Shi, *et al.*, Anatomy and nomenclature of tree shrew lymphoid tissues. *Experimental*  
390 *Animals* **71** (2), 173–183 (2022).
- 391 9. C. L. Nunn, Spleen size, disease risk and sexual selection: a comparative study in primates.  
392 *Evolutionary Ecology Research* **4** (1), 109–131 (2002).
- 393 10. D. R. Joseph, The ratio between the heart-weight and body-weight in various animals. *The*  
394 *Journal of experimental medicine* **10** (4), 521 (1908).
- 395 11. R. Hadek, The lymph nodes of the guinea-pig. *British Veterinary Journal* **107** (12), 487–  
396 493 (1951).
- 397 12. J. Kabat-Koperska, *et al.*, Changes in the immune system of female wistar rats after expo-  
398 sure to immunosuppressive treatment during pregnancy. *Scandinavian journal of immunol-*  
399 *ogy* **83** (6), 418–426 (2016).
- 400 13. M. Sarsilmaz, Y. Gumusalan, H. H. Celík, *et al.*, Classification of the thoracic and abdom-  
401 inal lymph nodes of the rat. *Turk J Med Res* **5**, 185–91 (1994).
- 402 14. R. Jackson, R. S. Morris, A study of the topography of the lymphatic system of the  
403 Australian brushtail possum (*Trichosurus vulpecula*). *Journal of anatomy* **188** (Pt 3), 603  
404 (1996).
- 405 15. A.-A. Dunne, *et al.*, Lymph node topography of the head and neck in New Zealand White  
406 rabbits. *Laboratory animals* **37** (1), 37–43 (2003).



- 407 16. S. Hamaguchi, *et al.*, Selective hyperthermia using magnetoliposomes to target cervical  
408 lymph node metastasis in a rabbit tongue tumor model. *Cancer science* **94** (9), 834–839  
409 (2003).
- 410 17. C. U. Herborn, *et al.*, Interstitial MR lymphography with MS-325: characterization of nor-  
411 mal and tumor-invaded lymph nodes in a rabbit model. *American Journal of Roentgenology*  
412 **179** (6), 1567–1572 (2002).
- 413 18. A. M. Seacat, *et al.*, Subchronic toxicity studies on perfluorooctanesulfonate potassium salt  
414 in cynomolgus monkeys. *Toxicological Sciences* **68** (1), 249–264 (2002).
- 415 19. A. Moriyama, *et al.*, Quantitative Analyses of Lymphoid Tissue in the Spleen, Lymph  
416 Nodes, and Peyer’s Patches in Cynomolgus Monkeys. *Journal of Veterinary Medical Sci-*  
417 *ence* pp. 1107110573–1107110573 (2011).
- 418 20. N. Anna Toenjes, *Felis catus* (On-line), *Animal Diversity Web* (2014 (accessed Nov 24,  
419 2020)), [https://animaldiversity.org/accounts/Felis\\_catus/](https://animaldiversity.org/accounts/Felis_catus/).
- 420 21. M. H. Ratzlaff, The superficial lymphatic system of the cat. *Lymphology* **3** (4), 151–159  
421 (1970).
- 422 22. E. Schreurs, *et al.*, Ultrasonographic anatomy of abdominal lymph nodes in the normal cat.  
423 *Veterinary Radiology & Ultrasound* **49** (1), 68–72 (2008).
- 424 23. R. Degabriele, T. Dawson, Metabolism and heat balance in an arboreal marsupial, the koala  
425 (*Phascolarctos cinereus*). *Journal of comparative physiology* **134** (4), 293–301 (1979).
- 426 24. J. J. Hanger, T. J. Heath, Topography of the major superficial lymph nodes and their efferent  
427 lymph pathways in the koala (*Phascolarctos cinereus*). *Journal of anatomy* **177**, 67 (1991).

- 428 25. P. Flood, The Anatomy of the Domestic Animals. *Australian Veterinary Journal* **60** (1983),  
429 doi:10.1111/j.1751-0813.1983.tb09599.x.
- 430 26. F. M. D. O. E. Silva, *et al.*, Morphological analysis of lymph nodes in odontocetes from  
431 north and northeast coast of Brazil. *The Anatomical Record* **297** (5), 939–948 (2014).
- 432 27. S. C. Walpole, *et al.*, The weight of nations: an estimation of adult human biomass. *BMC*  
433 *public health* **12** (1), 439 (2012).
- 434 28. B. Ogassavara, R. R. Tucunduva Neto, R. R. d. Souza, M. J. Tucunduva, Ultrasound eval-  
435 uation of the morphometric patterns of lymph nodes of the head and neck in young and  
436 middle-aged individuals. *Radiologia brasileira* **49** (4), 225–228 (2016).
- 437 29. S. M. Qatarnah, I.-C. Kiricuta, A. Brahme, U. Tiede, B. K. Lind, Three-dimensional atlas of  
438 lymph node topography based on the visible human data set. *The Anatomical Record Part*  
439 *B: The New Anatomist: An Official Publication of the American Association of Anatomists*  
440 **289** (3), 98–111 (2006).
- 441 30. J. Magilton, K. Tanudimadja, N. Ghoshal, The Lymph Nodes and Lymph Vessels of the  
442 Thoracic Viscera of the Goat (*Capra hircus*) 1. *Anatomia, Histologia, Embryologia* **2** (4),  
443 316–326 (1973).
- 444 31. L. Saar, Lymph nodes of the head, neck and shoulder region of swine. *Iowa State University*  
445 *Veterinarian* **25** (3), 3 (1962).
- 446 32. L. Saar, R. Getty, The lymph nodes and the lymph vessels of the abdominal wall, pelvic  
447 wall and the pelvic limb of swine. *Iowa State University Veterinarian* **26** (2), 9 (1963).

- 448 33. D. Rahmoun, M. Lieshchova, M. Fares, Morphological and radiological study of lymph  
449 nodes in dromedaries in Algeria. *Regulatory Mechanisms in Biosystems* **11** (2), 330–337  
450 (2020).
- 451 34. P. Gavrylin, D. Rahmoun, M. Lieshchova, H. Benchadi, Features topography and  
452 macrostructure of lymph nodes in Camels (*Camelus dromedarius*). *Online Journal of Ani-  
453 mal and Feed Research* **3** (2) (2013).
- 454 35. P. G. Jackson, P. D. Cockcroft, S. Elmhurst, *et al.*, *Clinical examination of farm animals*,  
455 i9780632057061 (Wiley Online Library, Online) (2002).
- 456 36. P. L. Altman, D. S. Dittmer, *et al.*, *Biology data book*, volume III. (1974).
- 457 37. H. Aijima, H. Hara, T. Harada, H. Hoshi, Histological Findings of the Lymph Nodes in a  
458 Case of an African Elephant. *Journal of Nihon University Medical Association* **77**, 19–22  
459 (2018), doi:10.4264/numa.77.1\_19.
- 460 38. V. Chatzaraki, *et al.*, Spleen measurements with reference to cause of death and spleen  
461 weight estimation: A study on postmortem computed tomography. *Journal of Forensic  
462 Radiology and Imaging* **18**, 24–31 (2019).
- 463 39. L. Schwartz, *et al.*, Evaluation of lymph nodes with RECIST 1.1. *European journal of  
464 cancer* **45** (2), 261–267 (2009).
- 465 40. A. J. De Langen, P. Raijmakers, I. Riphagen, M. A. Paul, O. S. Hoekstra, The size of  
466 mediastinal lymph nodes and its relation with metastatic involvement: a meta-analysis.  
467 *European journal of cardio-thoracic surgery* **29** (1), 26–29 (2006).

- 468 41. B. Ogassavara, R. R. Tucunduva Neto, R. R. d. Souza, M. J. Tucunduva, Ultrasound eval-  
469 uation of the morphometric patterns of lymph nodes of the head and neck in young and  
470 middle-aged individuals. *Radiologia brasileira* **49** (4), 225–228 (2016).
- 471 42. A. S. Perelson, F. W. Wiegel, Scaling aspects of lymphocyte trafficking. *Journal of theoret-*  
472 *ical biology* **257** (1), 9–16 (2009).
- 473 43. A. S. Perelson, G. F. Oster, Theoretical studies of clonal selection: minimal antibody  
474 repertoire size and reliability of self-non-self discrimination. *Journal of theoretical biol-*  
475 *ogy* **81** (4), 645–670 (1979).
- 476 44. F. W. Wiegel, A. S. Perelson, Some scaling principles for the immune system. *Immunology*  
477 *and cell biology* **82** (2), 127–131 (2004).
- 478 45. T. P. Arstila, *et al.*, A direct estimate of the human  $\alpha\beta$  T cell receptor diversity. *Science*  
479 **286** (5441), 958–961 (1999).
- 480 46. A. Casrouge, *et al.*, Size estimate of the  $\alpha\beta$  TCR repertoire of naive mouse splenocytes.  
481 *The Journal of Immunology* **164** (11), 5782–5787 (2000).
- 482 47. U. G. Wagner, K. Koetz, C. M. Weyand, J. J. Goronzy, Perturbation of the T cell repertoire  
483 in rheumatoid arthritis. *Proceedings of the National Academy of Sciences* **95** (24), 14447–  
484 14452 (1998).
- 485 48. I. Ionita-Laza, C. Lange, N. M. Laird, Estimating the number of unseen variants in the  
486 human genome. *Proceedings of the National Academy of Sciences* **106** (13), 5008–5013  
487 (2009).
- 488 49. H. Akaike, A new look at the statistical model identification. *IEEE transactions on auto-*  
489 *matic control* **19** (6), 716–723 (1974).

50. S. Celli, *et al.*, How many dendritic cells are required to initiate a T-cell response? *Blood, The Journal of the American Society of Hematology* **120** (19), 3945–3948 (2012).
51. J. Ferdous, G. Matthew Fricke, M. E. Moses, More Is Faster: Why Population Size Matters in Biological Search. *Journal of Computational Biology* **31** (5), 429–444 (2024), pMID: 38754139, doi:10.1089/cmb.2023.0296, <https://doi.org/10.1089/cmb.2023.0296>.
52. S. Luke, G. C. Balan, L. Panait, C. Cioffi-Revilla, S. Paus, MASON: A Java multi-agent simulation library, in *Proceedings of Agent 2003 Conference on Challenges in Social Simulation*, vol. 9 (2003).
53. G. M. Fricke, K. A. Letendre, M. E. Moses, J. L. Cannon, Persistence and adaptation in immunity: T cells balance the extent and thoroughness of search. *PLoS Computational Biology* **12** (3), e1004818 (2016).
54. R. J. De Boer, *et al.*, Recruitment times, proliferation, and apoptosis rates during the CD8+ T-cell response to lymphocytic choriomeningitis virus. *Journal of virology* **75** (22), 10663–10669 (2001).
55. S. Banerjee, M. Moses, Scale invariance of immune system response rates and times: perspectives on immune system architecture and implications for artificial immune systems. *Swarm Intelligence* **4** (4), 301–318 (2010).
56. C. J. Downs, N. A. Dochtermann, R. Ball, K. C. Klasing, L. B. Martin, The effects of body mass on immune cell concentrations of mammals. *The American Naturalist* **195** (1), 107–114 (2020).
57. C. L. Althaus, Of mice, macaques and men: scaling of virus dynamics and immune responses. *Frontiers in Microbiology* **6**, 355 (2015).

- 513 58. E. Cornelius Ruhs, *et al.*, Body size affects immune cell proportions in birds and non-volant  
514 mammals, but not bats. *Journal of Experimental Biology* **224** (13), jeb241109 (2021).
